# Supplementary material for: Predictor-corrector algorithms for stochastic optimization under gradual distribution shift
Source: arXiv:2205.13575 source file (2023-02-23)
Supplement: Supplementary file 1 [file Supp_applications.tex]

In this section we present some other applications, where we establish the superiority of the performance of the predictor-corrector method. 
\subsection{Performative prediction}
\label{sec:performative}
In this subsection we present another example for performative prediction problem along the line of the example presented in Section 4.1 of \cite{mendler2020stochastic} in a time-varying format as elaborated in Section 5.1 of \cite{cutler2021stochastic}. The setup is as follows: suppose $Z \sim \cD(\theta) \triangleq \cN(\mu + \eps \theta, \sigma^2)$ and $\ell(Z, \theta) = 0.5(Z - \theta)^2$. Then the performative optimal solution of this problem: 
$$
\theta_{PO} = \argmin_{\theta} \cR(\theta) = \argmin_{\theta} \bbE_{Z \sim \cD(\theta)}\left[\ell(Z, \theta)\right] = \frac{\mu}{1 - \eps} \,.
$$
To extend this problem into a time varying setup, assume that by $\mu$ and $\eps$ changes with time. As elaborated in \cite{mendler2020stochastic}, we assume for stability $\eps(t) \in (0, 1)$. The time-varying risk function is then defined as: 
$$
\cR(\theta, t) = \bbE_{Z \sim \cD(\theta, t)}\left[\ell(Z, \theta)\right]
$$
where $\cD(\theta, t) = \cN(\mu(t) + \eps(t) \theta, \sigma^2)$. Consequently, $\theta^\star_t$ is defined as the performatively optimal solution at time $t$, i.e. 
$$
\theta^\star_t = \argmin_{\theta}\cR(\theta, t) = \frac{\mu(t)}{1 - \eps(t)}. 
$$
We aim to estimate/track this $\theta^\star_t$ using both gradient descent and predictor-corrector method. As mentioned in the previous example, we need to estimate gradient and Hessian of $\cR(\theta, t)$ with respect to $\theta$ and the time derivative of gradient. For simplicity of the exposition, we assume that we can query the derivatives of the normal density (i.e. gradient, Hessian with respect to $\theta$ and time derivative of the gradient).
More precisely, suppose $\phi_{\theta, t}$ denotes the density of $\cD(\theta, t)$, i.e. normal density with mean $\mu(t) + \eps(t)\theta$ and variance $\sigma^2$. Then, we assume that $\phi_{\theta, t}$, $\nabla_\theta \phi_{\theta, t}, \nabla_{\theta \theta} \phi_{\theta, t}$ and $\nabla_{\theta t} \phi_{\theta, t}$ can be evaluated at any point. Assume that at time $t$, we have $n$ samples $Z^t_1,\dots, Z^t_n \sim \cD(t, \theta^*_t)$. The gradient of risk function at time $t$ is: 
\begin{align*}
\nabla_\theta R(\theta, t) & = \bbE_{Z \in \cD(\theta, t)}\left[\nabla_\theta \ell(Z, \theta)\right] + \bbE_{Z \in \cD(\theta, t)}\left[\ell(Z, \theta)\frac{\nabla_\theta \phi_{\theta, t}(Z)}{\phi_{\theta, t}(Z)}\right] \\
& = -\bbE_{Z \in \cD(\theta, t)}[Z] + \theta + \frac12  \bbE_{Z \in \cD(\theta, t)}\left[(Z - \theta)^2\frac{\nabla_\theta \phi_{\theta, t}(Z)}{\phi_{\theta, t}(Z)}\right] 
\end{align*}
We can estimate the gradient by the sample average based on the data $\{Z_j^t\}_{j=1}^n$. For the Hessian, we follow a similar route: 
\begin{align*}
    \nabla_{\theta\theta} R(\theta, t)  & = \bbE_{Z \in \cD(\theta, t)}\left[\nabla_{\theta\theta} \ell(Z, \theta)\right] + \bbE_{Z \in \cD(\theta, t)}\left[\nabla_\theta \ell(Z, \theta)\frac{\nabla_\theta \phi_{\theta, t}(Z)}{\phi_{\theta, t}(Z)}^{\top}\right] \\
    & \qquad \qquad +  \bbE_{Z \in \cD(\theta, t)}\left[\frac{\nabla_\theta \phi_{\theta, t}(Z)}{\phi_{\theta, t}(Z)}\nabla_\theta \ell(Z, \theta)^{\top}\right] + \bbE_{Z \in \cD(\theta, t)}\left[\ell(Z, \theta)\frac{\nabla_{\theta\theta} \phi_{\theta, t}(Z)}{\phi_{\theta, t}(Z)}\right] \\
    & = 1 + \bbE_{Z \in \cD(\theta, t)}\left[(\theta - Z)\frac{\nabla_\theta \phi_{\theta, t}(Z)}{\phi_{\theta, t}(Z)}^{\top}\right] + \bbE_{Z \in \cD(\theta, t)}\left[\frac{\nabla_\theta \phi_{\theta, t}(Z)}{\phi_{\theta, t}(Z)}(\theta - Z)^{\top}\right]  \\
    & \hspace{19em} + \bbE_{Z \in \cD(\theta, t)}\left[(Z - \theta)^2\frac{\nabla_{\theta\theta} \phi_{\theta, t}(Z)}{\phi_{\theta, t}(Z)}\right] \\
    & = 1 - 2\bbE_{Z \in \cD(\theta, t)}\left[Z\frac{\nabla_\theta \phi_{\theta, t}(Z)}{\phi_{\theta, t}(Z)}\right] +  \bbE_{Z \in \cD(\theta, t)}\left[(Z - \theta)^2\frac{\nabla_{\theta\theta} \phi_{\theta, t}(Z)}{\phi_{\theta, t}(Z)}\right] 
\end{align*}
Therefore, we can also estimate the Hessian based on the sample average with the data $\{Z_j^t\}_{j=1}^n$. Analysis of the time derivative of the gradient is similar: 
\begin{align*}
    \nabla_{\theta t} R(\theta, t) & = \bbE_{Z \in \cD(\theta, t)}\left[\nabla_\theta \ell(Z, \theta)\frac{\nabla_t \phi_{\theta, t}(Z)}{\phi_{\theta, t}(Z)}\right] + \bbE_{Z \in \cD(\theta, t)}\left[\ell(Z, \theta)\frac{\nabla_{\theta t} \phi_{\theta, t}(Z)}{\phi_{\theta, t}(Z)}\right] \\
    & = \bbE_{Z \in \cD(\theta, t)}\left[(\theta - Z)\frac{\nabla_t \phi_{\theta, t}(Z)}{\phi_{\theta, t}(Z)}\right] + \bbE_{Z \in \cD(\theta, t)}\left[(\theta - Z)^2\frac{\nabla_{\theta t} \phi_{\theta, t}(Z)}{\phi_{\theta, t}(Z)}\right] \\
    & = -\bbE_{Z \in \cD(\theta, t)}\left[Z\frac{\nabla_t \phi_{\theta, t}(Z)}{\phi_{\theta, t}(Z)}\right] + \bbE_{Z \in \cD(\theta, t)}\left[(\theta - Z)^2\frac{\nabla_{\theta t} \phi_{\theta, t}(Z)}{\phi_{\theta, t}(Z)}\right] 
\end{align*}
which can again be estimated from the sample average.
